# Supplementary material for: Modularizing Behavioral and Architectural Crosscutting Concerns in Formal Component-Based Systems - Application to the Behavior Interaction Priority Framework
Source: arXiv:1805.08406 source file (2018-05-22)
Supplement: Supplementary file 2 [file appendix.tex]

\subsection{Interference}
\begin{example}
Figure \ref{fig:interfere} displays the multiple weaving scenarios of two aspects $asp_1$ and $asp_2$ where:
\begin{itemize}
	\item $asp_1 = \tuple{B, pc, \setof{}, F_b, F_a, \setof{}}$
	\item $asp_2 = \tuple{B, pc, \setof{}, F'_b, F'_a, \setof{}}$
\end{itemize}
Both aspects share the same pointcut $pc = \setof{\pcloc(\ell_1), \pcportexec(p_1)}$.
Let $t_1$ be the transition guarded by $g_1$ labeled by $p_1$ and whose computation is $f_1$.
Both aspects will share the same match: $m = \tuple{\setof{t_1}, \WCurrentBefore, \WCurrentAfter}$.
According to the execution frame both $F_b$ and $F'_b$ must be prepended to $f_1$.
$F_a$ and $F'_a$ must be appended to $f_1$.
The four scenarios display the possible arrangements to order $F_b$, $F_b'$, $F_a$ and $F'_a$.
The order would not be an issue if all those functions do not write to the component variables.
For example in the case of logging, the ordering would not matter.
However suppose $F_b = \ffunc[x := 3]$ and $F'_b = \ffunc[x := 2]$.
The variable $x$ will be changed to either $3$ or $2$ by the end of the before section.
This causes the original computation $f_1$ to behave non-deterministically if it depends on $x$.
\end{example}
\getexamples[interfere]{example-inter1, example-inter2, example-inter3, example-inter4}
			{Interference In Atomic Components}{0.8}{2}
